# Supplementary material for: PILLOW: Enhancing Efficient Instruction Fine-tuning via Prompt Matching
Source: arXiv:2312.05621 source file (2024-10-07)
Supplement: Supplementary file 2 [file reward_type.tex]

\section{Reward Type}
\label{sec:reward_type}

We also ablate on the reward type, i.e. continuous or discrete. Given the calculated score $\kappa$, for the continuous reward, we define the calculation as:
\begin{equation}
    r = \alpha \cdot \kappa,
\end{equation}
and for the discrete reward, we define it as:

\begin{equation}
    r = \left\{
    \begin{aligned}
        \alpha \cdot \kappa, ~&\kappa >= 0.6\\
        0, ~&\mathrm{else} \\
    \end{aligned}
    \right.
\end{equation}

We observe that discrete rewards make RL training unstable. As shown in Figure ?,
